# Supplementary material for: Inference Attacks Against Face Recognition Model without Classification Layers
Source: arXiv:2401.13719 source file (2024-01-24)
Supplement: Supplementary file 1 [file X_suppl.tex]

\clearpage
\setcounter{page}{1}
\maketitlesupplementary
% \usepackage[section]{placeins}

% \section{Rationale}
% \label{sec:rationale}
% % 
% Having the supplementary compiled together with the main paper means that:
% % 
% \begin{itemize}
% \item The supplementary can back-reference sections of the main paper, for example, we can refer to \cref{sec:intro};
% \item The main paper can forward reference sub-sections within the supplementary explicitly (e.g. referring to a particular experiment); 
% \item When submitted to arXiv, the supplementary will already included at the end of the paper.
% \end{itemize}
% % 
% To split the supplementary pages from the main paper, you can use \href{https://support.apple.com/en-ca/guide/preview/prvw11793/mac#:~:text=Delete%20a%20page%20from%20a,or%20choose%20Edit%20%3E%20Delete).}{Preview (on macOS)}, \href{https://www.adobe.com/acrobat/how-to/delete-pages-from-pdf.html#:~:text=Choose%20%E2%80%9CTools%E2%80%9D%20%3E%20%E2%80%9COrganize,or%20pages%20from%20the%20file.}{Adobe Acrobat} (on all OSs), as well as \href{https://superuser.com/questions/517986/is-it-possible-to-delete-some-pages-of-a-pdf-document}{command line tools}.

\section{Comparsion of Feature Distances for the Member and Non-member}
\label{sec:rationale}
In this section, we give more details of experiments about the distance distribution comparison. We use a widespread network IR-SE-50 \cite{he2016deep,hu2018squeeze} as the backbone, which consists of an input layer, an output layer and 4 sub-blocks. 
% It is worth noting that most of  well-known Resnet and its variants have the similar architecture. 
We extract the parameters "running mean" and "running var" in the last BatchNorm2d layer of each sub-block. In the backbone, the input and output layers include a BatchNorm2d layer separately. Besides, the output layer also has a BatchNorm1d layer. That is to say, we can obtain the parameters totally from 6 BatchNorm2d layers and 1 BatchNorm1d layer, and all the parameters are 1-dimensional vectors, denoted as $u \in R^{1\times c} $. We represent the "running mean" and "running var" as $u_{mean}$ and $u_{var}$,  respectively.

When computing the distance between the feature mean (or the feature) and "running mean", we average the intermediate feature  $v_{2d} \in R^{1\times c\times h \times w}$ (the feature before a BatchNorm2d layer) for the dimensions $h \times w$ and obtain the feature mean $\overline{v}_{2d} \in R^{1\times c}$. Then we can compute the distance between $\overline{v}_{2d}$ and $u_{mean}$ using Eq.2 in the paper. And the intermediate features before a BatchNorm1d layer, denoted as $v_{1d} \in R^{1\times c}$, have the same size as that of $u_{mean}$, so we can directly obtain the distance using Eq.2. And 7 distances are shown in Fig.\ref{mean} .

Note that we also 
compute the distance between the feature \emph{variance} and "running var" $u_{var}$.
% compare the \emph{variance} of the feature with $u_{var}$ when computing the distance between features and "running var". 
Specifically, we calculate the variance of $v_{2d} \in R^{1\times c\times h \times w}$ for the dimensions $h \times w$ 
% along both the height and width dimensions 
and obtain the feature \emph{variance} $\hat{v}_{2d} \in R^{1\times c}$, and then compute the distance as above. However, it makes no sense that we directly compute the distance between the variance of the feature before the BatchNorm1d layer and the corresponding $u_{var} \in R^{1\times c}$. Since $u_{var}$ in the BatchNorm1d layer is obtained by calculating the variance of a batch of features along only the batch dimension $B$. Despite the size of the feature $v_{1d} \in R^{1\times c}$ being the same as that of $u_{var}$, it does not provide any physical meaning if we perform mathematical operations on them directly. Therefore, we abandon the distance about the intermediate feature $v_{1d}$ and "running var", and obtain 6 distances as shown in Fig.\ref{var} .

\section{Membership Inference Attack}
In the paper, we use CASIA-WebFace \cite{yi2014learning} as the training dataset in the case 1. When training and testing the attack model, we sample face images from another dataset as the non-members. Here we give a more challenging case. We split the one dataset $\mathcal{D}$ (CASIA-WebFace) by half into $\mathcal{D}^{member}$ and $\mathcal{D}^{non-member}$. And then we split $\mathcal{D}^{member}$ into $\mathcal{D}_{train}^{member}$ and $\mathcal{D}_{test}^{member}$. $\mathcal{D}_{train}^{member}$ is used to train the attack model and $\mathcal{D}_{test}^{member}$ for the test. We perform the same operation on $\mathcal{D}^{non-member}$ and obtain $\mathcal{D}_{train}^{non-member}$,  $\mathcal{D}_{test}^{non-member}$. We also use different proportions of the dataset for training the attack model and the number of testing images is 60,000. Furthermore, we perform extended experiments with additional settings for ablation study. Besides the settings mentioned in the paper, we replace "mean distance" with "variance distance", in which case the attack model takes only "variance distance" as the input and the images are not flipped, denoted as $\mathcal{A}_{var}$. We also consider the case where both "mean distance" and "variance distance" are the input and the images are flipped, denoted as $\mathcal{A}_{mean\&var\&flip}$. We show the results in Tab.\ref{table1}. 
We find the attack success rate of the $\mathcal{A}_{var}$ case is lower than that of the $\mathcal{A}_{mean}$ case. In the cases without 'FR(flip)', the attack success rates of $\mathcal{A}_{mean\&var\&flip}$ and $\mathcal{A}_{mean\&flip}$ are similar. 
But in the cases with 'FR(flip)', the attack success rate of $\mathcal{A}_{mean\&var\&flip}$ is lower than that of $\mathcal{A}_{mean\&flip}$. 
From the above results, it can be seen that the introduction of $\mathcal{A}_{var}$ did not bring more performance gains. Therefore, in the experiments of the paper, we did not consider the case using $\mathcal{A}_{var}$.
% There exist some cases where the attack success rate of $\mathcal{A}_{mean\&var\&flip}$ is marginally higher than $\mathcal{A}_{mean\&flip}$. We think it is because "running var" cause a perturbation, as the model taking "running var" alone as the input does not give a expected result (see the performance of "$\mathcal{A}_{var}$").

\section{Model Inversion Attack}
We provide more results of our model inversion attack algorithm as shown in Fig\ref{fig1}. We try to reconstruct identities as many as possible, but find 
the number of reconstructed identities is less than the case with a classification layer.
% the number of recovered identities is limited. 
We believe that the main reason for this result is the lack of classification layers, which includes much privacy information. However, to our knowledge, this is the first time that the model inversion attack is launched against an FR model without the classification layer.

\newpage
% Despite we can generate images as variously as possible, experiments demonstrate that our generation is vulnerable to mode collapse. We think this results from the attack model, which may find a type of data that is easily predicted as a member and thus guide to generate that one type. That is why we can only reconstruct part certain identities of the training dataset and can not cover every identity during optimization.

\begin{figure*}[htbp]
  % \begin{minipage}{13cm}
  \centering
    \includegraphics[width=1.6\columnwidth]{./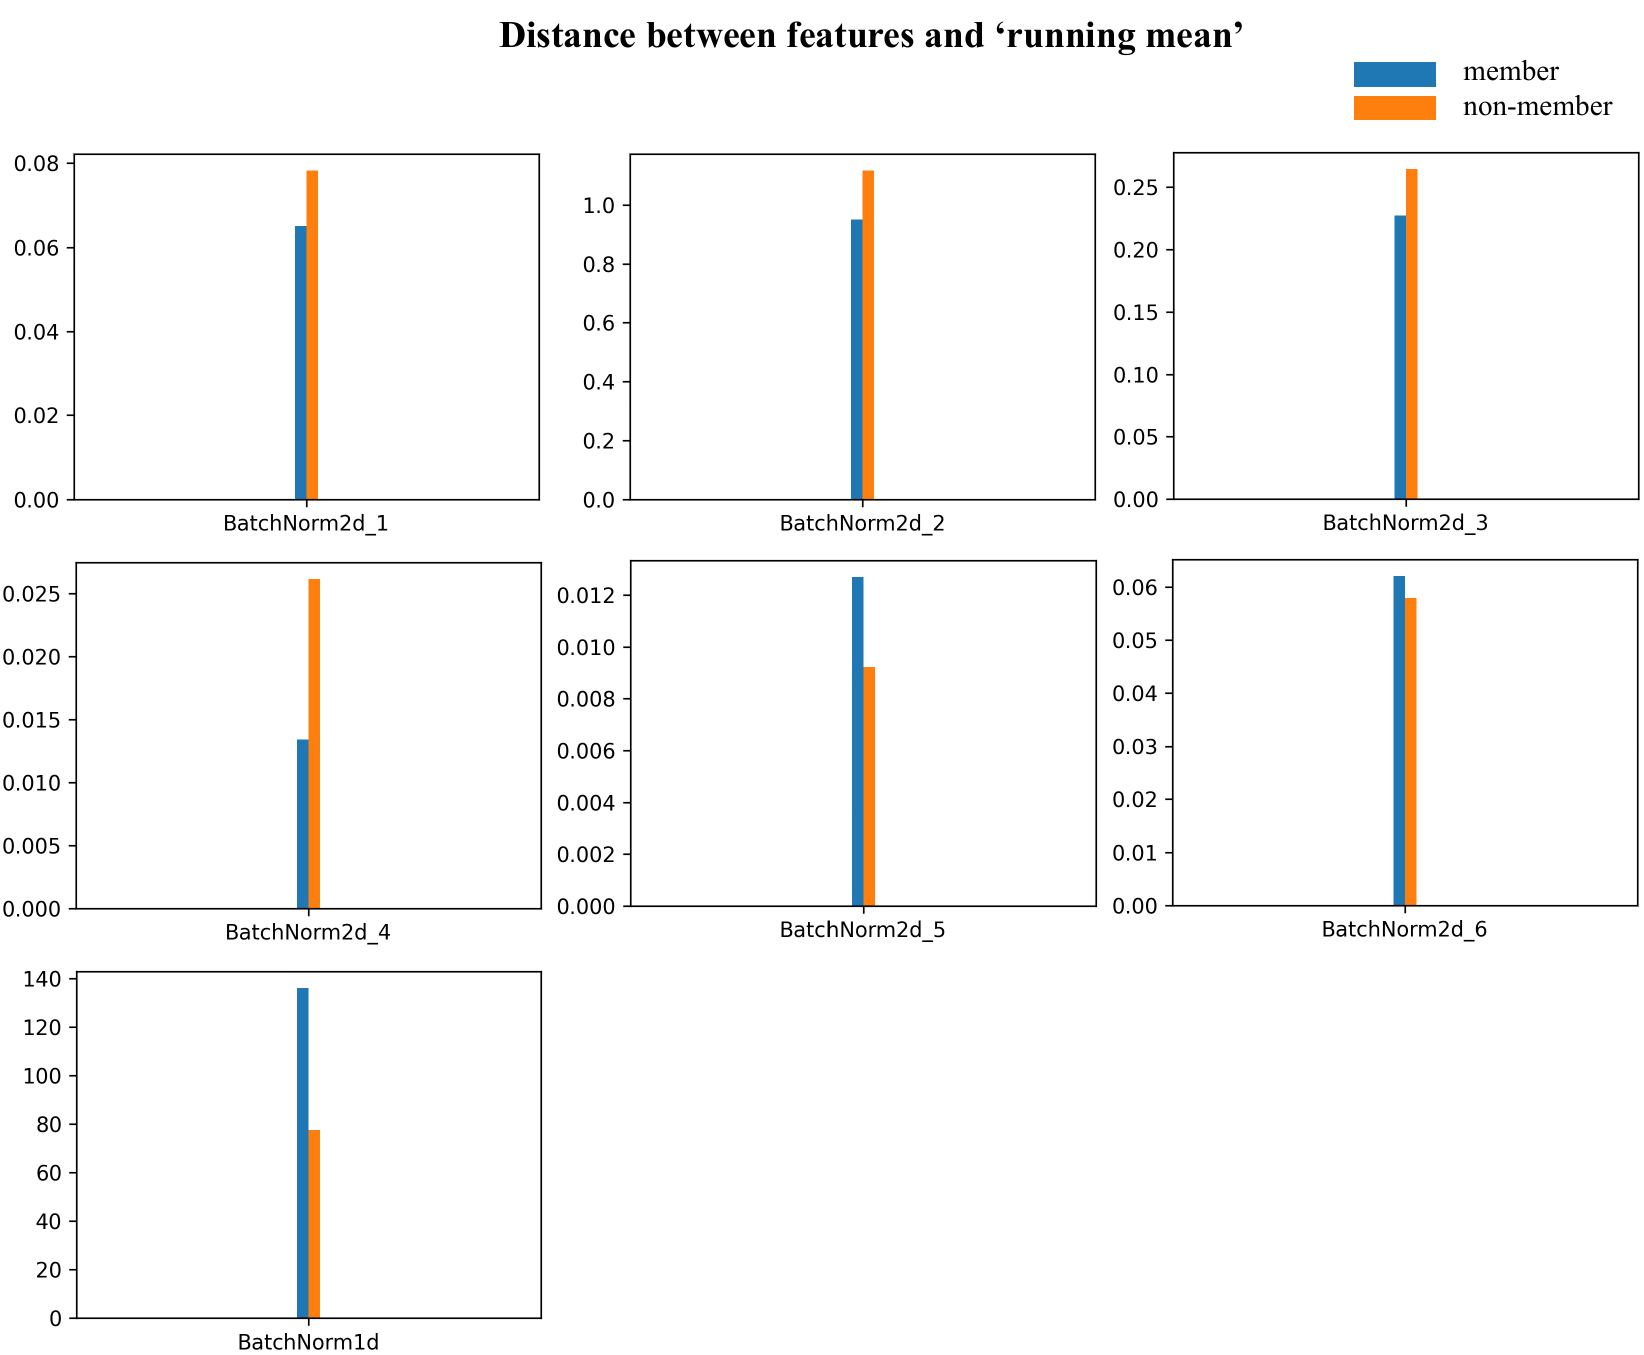}
  % \end{minipage}
  % \fbox{\rule[-.5cm]{0cm}{4cm} \rule[-.5cm]{4cm}{0cm}}
  \caption{Visualization of distances between the intermediate features and "running mean" for the Member and Non-member.}
  \label{mean}
\end{figure*}

\begin{figure*}[htbp]
  % \begin{minipage}{13cm}
  \centering
    \includegraphics[width=1.6\columnwidth]{./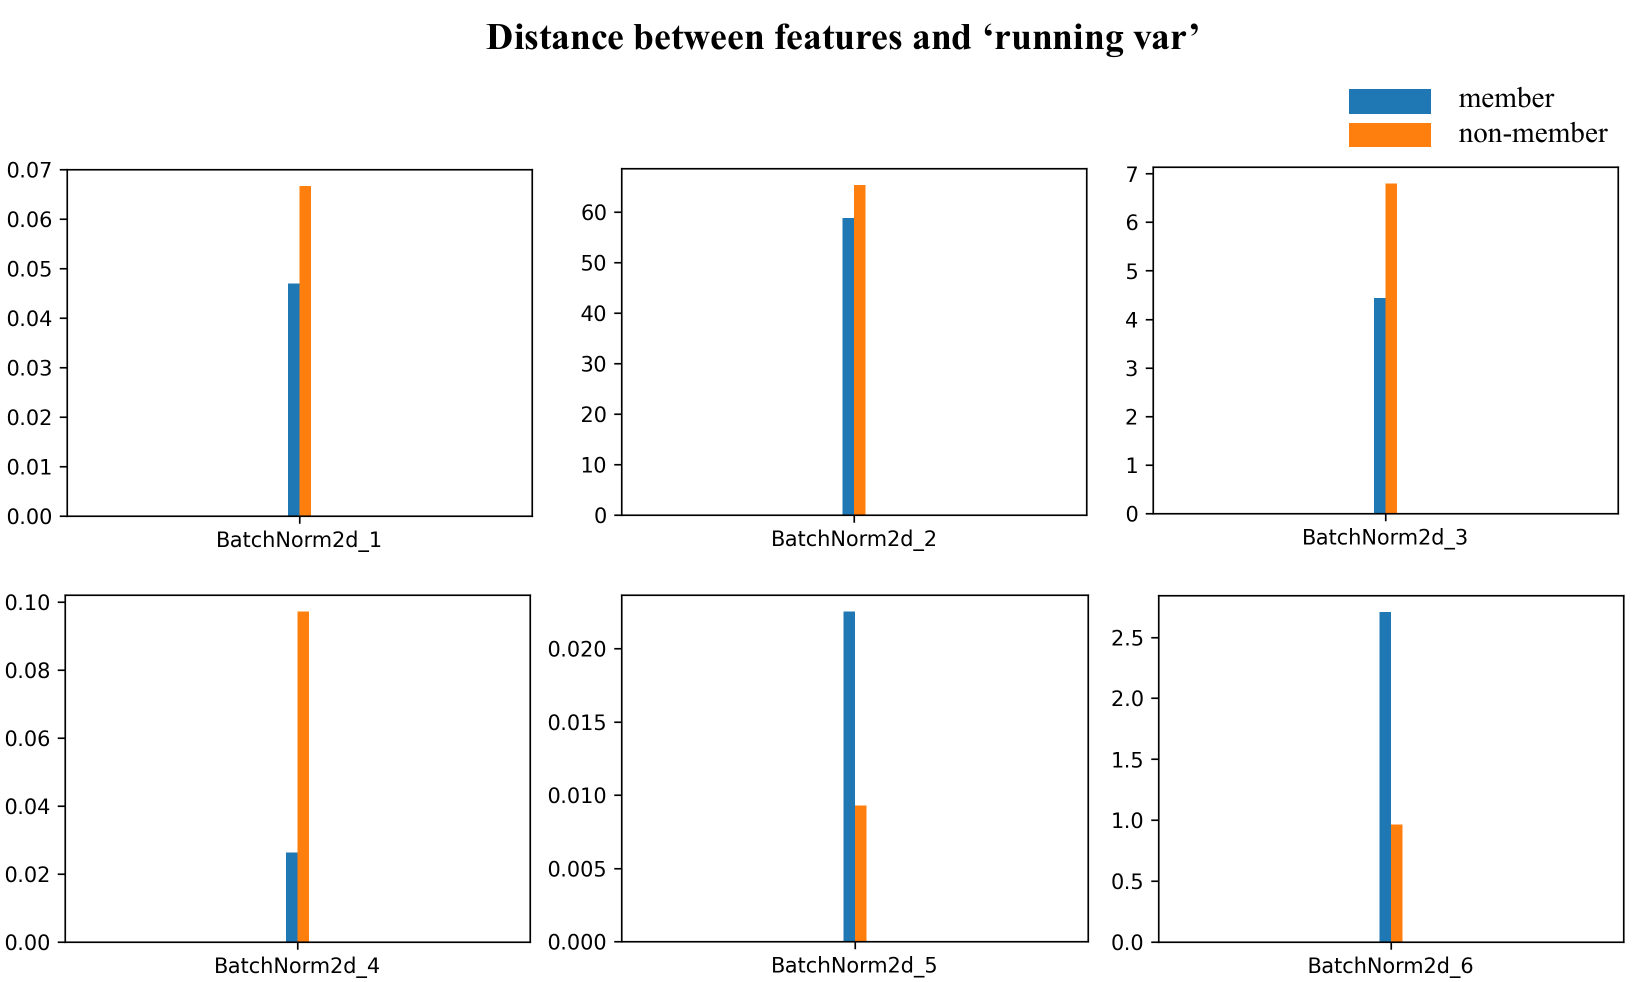}
  % \end{minipage}
  % \fbox{\rule[-.5cm]{0cm}{4cm} \rule[-.5cm]{4cm}{0cm}}
  \caption{Visualization of distances between the intermediate features and "running var" for the Member and Non-member.}
  \label{var}
\end{figure*}

\begin{table*}[htbp]
  \centering
  \begin{tabular}{ccccccc}
    \toprule
    \multirow{2}{*}[-0.1cm]{$\mathcal{D}_p$} & \multicolumn{6}{c}{Proportion}                   \\
    \cmidrule(r){2-7}
     & 1\%      & 5\% &10\% &1\%+FR(flip)& 5\%+FR(flip)&10\%+FR(flip)\\
    \midrule
    ASSD \cite{gao2022similarity}&57.89 & 59.76  & 59.63  &59.73  &58.95 &62.04\\
    $\mathcal{A}_{mean}$     &74.66     &75.96  &76.01  &71.82  &73.00 &73.29\\
    $\mathcal{A}_{var}$      &59.05      &60.60  &60.97 &57.78 &61.31 &62.47\\
    $\mathcal{A}_{mean\&var}$ &75.28      &75.99  &76.60 &71.98 &72.74 &73.21\\
    % $\mathcal{A}_{diff\_vec}$ &64.59        &63.26     &72.11   &79.11\\
    $\mathcal{A}_{mean\&flip}$ &\textbf{91.23}               &92.14       &92.82 &\textbf{87.22} &\textbf{86.81} &\textbf{87.33}\\
    $\mathcal{A}_{mean\&var\&flip}$ &90.91             & \textbf{92.28}      &\textbf{93.22} &83.31 &86.09 &87.20\\
    \bottomrule
  \end{tabular}
  \caption{The attack success rate of the membership inference attack in the case 1. We split the one dataset $\mathcal{D}$ (CASIA-WebFace) by half into $\mathcal{D}^{member}$ and $\mathcal{D}^{non-member}$. We also consider the case where the target models are trained with randomly flipped images, denoted as 'FR(flip)'.}
  \label{table1}
\end{table*}

\begin{figure*}[htbp]
  % \begin{minipage}{13cm}
  \centering
  \includegraphics[width=1.8\columnwidth]{./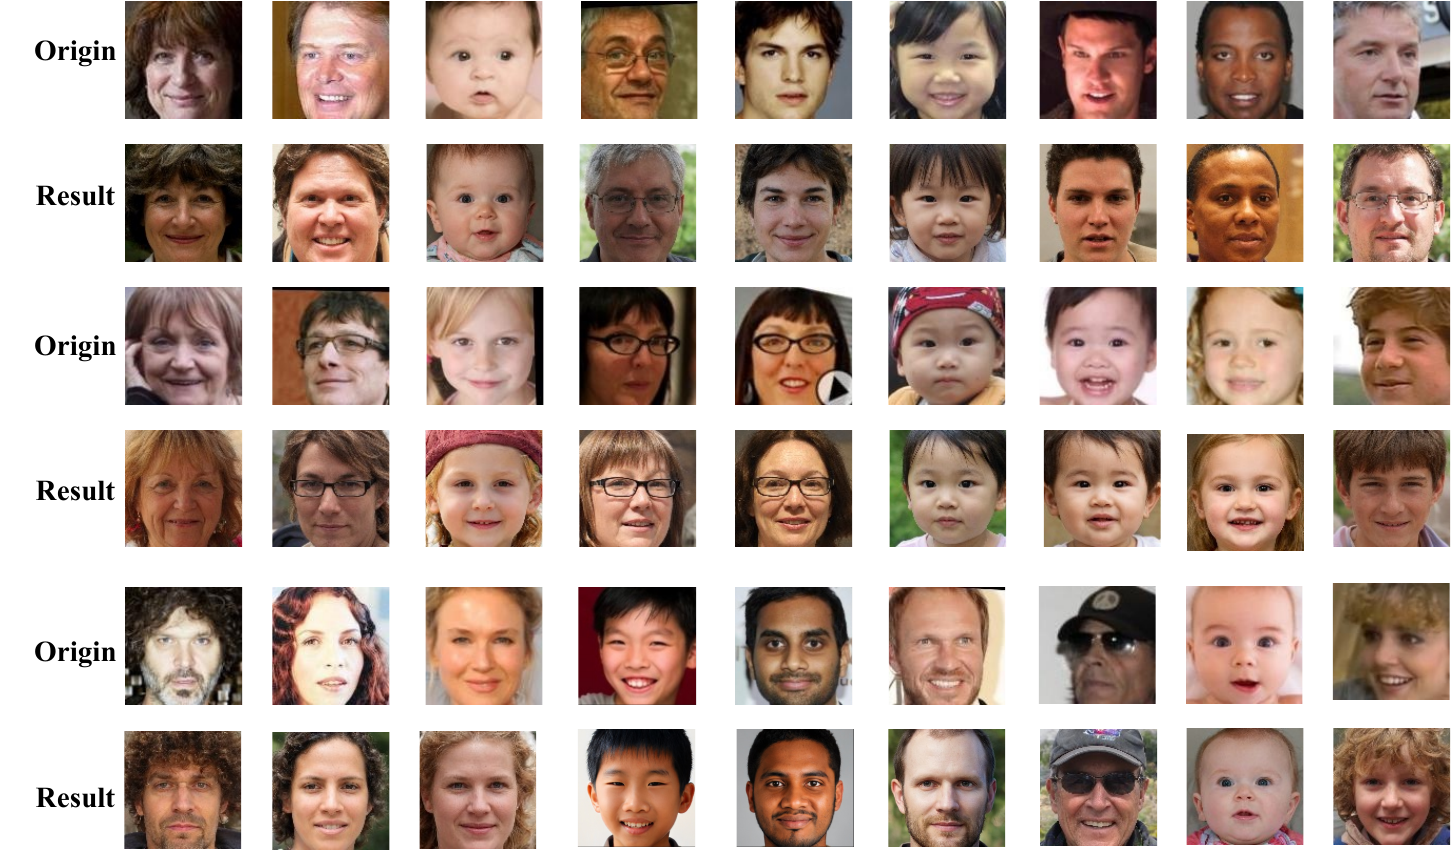}
  % \end{minipage}
  % \fbox{\rule[-.5cm]{0cm}{4cm} \rule[-.5cm]{4cm}{0cm}}
  \caption{More results of the model inversion attack in case 2.}
  \label{fig1}
\end{figure*}

% {
%     \small
%     \bibliographystyle{ieeenat_fullname}
%     \bibliography{main}
% }
